# Supplementary material for: Box-QAymo: Box-Referring VQA Dataset for Autonomous Driving
Source: arXiv:2507.00525 source file (2025-07-01)
Supplement: Supplementary file 1 [file appendix.tex]

\section{Research Methods}
